# Supplementary material for: Out-of-focus: Learning Depth from Image Bokeh for Robotic Perception
Source: arXiv:1705.01152 source file (2017-05-02)
Supplement: Supplementary file 1 [file 07_appendix.tex]

%-------------------------------------------------------------------------------------------------------------------------------------------------------------------
% Appendix
%-------------------------------------------------------------------------------------------------------------------------------------------------------------------

%-------------------------------------------------------------------------------------------------------------------------------------------------------------------
\subsection{Code Example 1}
\label{app:1}

%%%
\begin{lstlisting}
%% Code example 1
\end{lstlisting}
%%%
